# Supplementary material for: The Onset of Phase Separation in the Double Perovskite Oxide La$_2$MnNiO$_6$
Source: arXiv:1710.08535 source file (2018-04-15)
Supplement: Supplementary file 1 [file 10_18_17_LMNO_Interface_Supp_Final.pdf]

# The Onset of Phase Separation in the Double Perovskite Oxide $La_2MnNiO_6$

Steven R. Spurgeon,[1] Peter V. Sushko,[1] Arun Devaraj,[1] Yingge Du,[1] Timothy Droubay,[1] and Scott A. Chambers[1]

*Physical and Computational Sciences Directorate, Pacific Northwest National Laboratory, Richland, WA 99352, USA*

## SUPPLEMENTARY MATERIAL

### A. Experimental Methods

#### *1. Thin Film Synthesis*

As-received STO substrates ($10 \times 10 \times 0.5$ mm, MTI Corporation) were etched in buffered HF and annealed to ensure a $TiO_2$-terminated surface.[1] They were subsequently cleaned by heating in the MBE chamber at 650 °C for 20 min in an oxygen partial pressure of $6.0 \times 10^{-6}$ Torr prior to film growth. The LMNO thin films were grown on $SrTiO_3$ (001) substrates in a custom MBE system. La, Mn, and Ni were co-evaporated from high-temperature effusion cells and the evaporation rates were calibrated using a quartz crystal microbalance positioned at the substrate position prior to each growth. The substrate temperature during growth was varied from 600–750 °C, and 650 °C was determined to be the optimal condition for the growth of high quality films reported in this work. An activated oxygen plasma beam (with $O_2$ partial pressure in the chamber set at $\sim 1 \times 10^{-5}$ Torr) was incident on the sample during deposition. *In situ* RHEED was used to monitor the overall morphology and surface structure. After deposition, the substrate temperature was reduced at a rate of 30 °C min$^{-1}$ under the same oxygen environment. Two sectioned pieces of a 40 nm-thick LMNO film were post-annealed at 750 °C and 800 °C (3 °C min$^{-1}$ ramp rate up/down) for 2 hours in a tube furnace, respectively, to promote cation ordering. Detailed structural characterization is given elsewhere.[2]

#### *2. Scanning Transmission Electron Microscopy*

STEM samples were prepared using a lift-out method on an FEI Helios DualBeam Focused Ion Beam (FIB) operating at 2–30 keV and 5–7° incidence angle. STEM images were acquired along the STO [100] and [110] zone-axes using a JEOL ARM-200CF probe-corrected microscope operating at 200 keV, with the following probe convergence / collection inner / outer semi-angles: STEM-HAADF = 27.5 / 90–370 mrad, STEM-LAADF = 27.5 / 27–110 mrad, and STEM-ABF = 21 mrad / 10–23 mrad. Drift-corrected images were prepared using the SmartAlign[3] non-rigid alignment routine to improve signal-to-noise; for this, a series of 20 frames at $512 \times 512$ pixels with a fast 2 µs px$^{-1}$ dwell time was used.

### *3. X-ray Diffraction*

Lattice parameters and overall crystal quality were determined using high-resolution X-ray diffraction and reciprocal space mapping with a Philips X'Pert diffractometer equipped with a Cu anode ($\lambda = 1.54065$ Å) operating at 45 kV and 40 mA, a hybrid monochromator consisting of four-bounce double crystal Ge (220), and a Cu X-ray mirror. While the epitaxial relationship and an out-of-plane lattice parameter of 3.862 Å are derived from a $\theta - 2\theta$ scan, the RSM taken around the (103) film reflection shown in Figure **??**.C reveals that the film is coherent strained to the substrate in-plane.

### *4. Atom Probe Tomography*

APT needle samples were prepared using a lift-out method on FEI Helios and Quanta DualBeam Focused Ion Beams (FIBs) operating at 2–30 keV. The best results were obtained with the film-substrate interface oriented parallel to the APT needle axis.[4] The APT analysis was conducted using a CAMECA LEAP 4000XHR system with a 355 nm wavelength pulsed UV laser, using a 100 pJ laser pulse energy and 100 KHz pulse repetition rate, while maintaining the sample temperature at 50–60 K and evaporation rate at 0.003 atoms per pulse. The APT results were analyzed using the IVAS 3.6.8 software. 15 at % Ni iso-composition surfaces were subsequently generated to produce Figure **??**.

### *5. Density Functional Theory*

The ideal and defective $La_2MnNiO_6$ / $SrTiO_3$ systems were represented using the periodic slab model and a 2×2 lateral cell. The $SrTiO_3$ part of the slab contains four unit cells along the $c$-axis; the LMNO part contains up to four unit cells. The in-plane cell parameter was fixed at the value pre-calculated for the bulk $SrTiO_3$ (3.895 Å), while the $c$-parameter was set to 50 Å, which leaves the vacuum gap of at least 20 Å. The calculations were performed using the Vienna *Ab Initio* Simulation Package (VASP).[5,6] The projected augmented wave (PAW) method was used to approximate the core electron potential.[7] Exchange-correlation effects were treated within the Perdew-Burke-Ernzerhoff (PBE) functional form of the GGA, modified for solids (PBEsol).[8] The calculations were performed using a $2 \times 2 \times 1$ Monkhorst-Pack $k$-point mesh with its origin at the $\Gamma$-point. The charge and spin density distributions

were analyzed using the Bader method.[9] The total energy was minimized with respect to the internal coordinates. The energies of self-consistent calculations were converged to $10^{-5}$ eV cell$^{-1}$, and the atomic positions were relaxed until the forces on the ions were less than 0.02 eV Å$^{-1}$. The plane-wave basis with a 500 eV cutoff was used. Single point electronic structure calculations were performed using the GGA+$U$ scheme[10] for the pre-optimized structures in order to better represent localization of electron charge in oxygen deficient LMNO. For simplicity, the same value of $U$=5.0 eV was applied to $3d$ states of all transition metals. This value is close to $U_{\mathrm{Mn}} = 5.25$ eV and $U_{\mathrm{Ni}} = 5.77$ eV used for $Mn^{4+}$ and $Ni^{2+}$, respectively.[11]

## B. Comparison of HAADF and LAADF for NiO Precipitate Visualization

As described in the main text, the observed nanoscale precipitates are difficult to detect, particularly deeper into the film where the TEM foil is generally thicker. However, there is a sizable strain field associated with the precipitates, which is more easily visualized using more coherent imaging modes, such as low-angle annular dark field (STEM-LAADF). In Figure S1 we show a comparison between STEM-HAADF and STEM-LAADF images taken from similar regions of the film; while some contrast modulation is present in the former, the extensive network of precipitates is readily apparent in the latter.

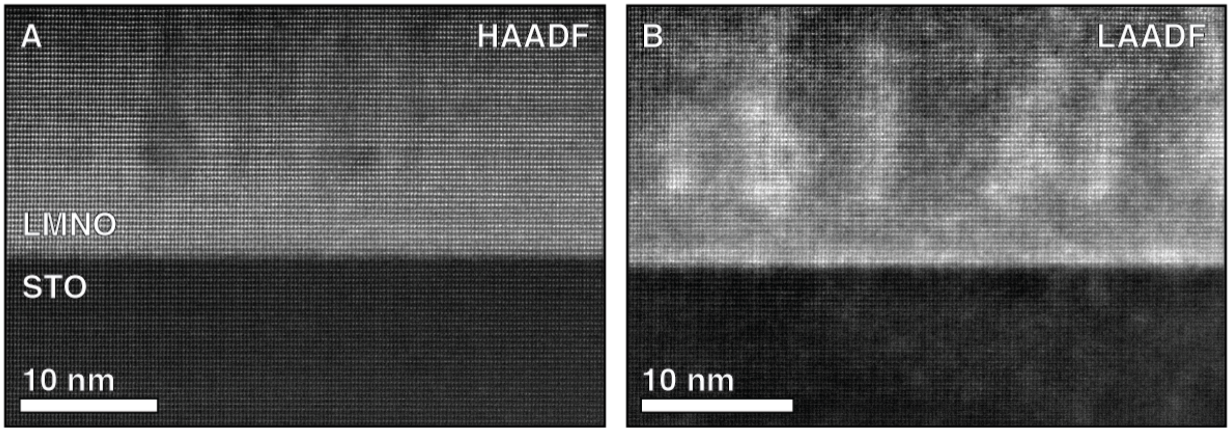


FIG. S1. Comparison of (A) STEM-HAADF and (B) STEM-LAADF images taken from similar film regions to illustrate the effect of imaging mode on precipitate visualization.

## C. Chemical Mapping of the Precipitate Environment

We have performed local STEM-EELS composition mapping around a representative NiO / LMNO interface, as shown in Figure S2. We observe a clear composition gradient from the particle to the matrix, as confirmed by APT, as well a Mn enrichment around the core of the NiO. This finding supports the partitioning of Mn and Ni during film growth. To confirm the conclusions of our DFT simulations, we have investigated the Mn $L_{23}$ edge fine structure in the vicinity of a NiO precipitate. Figure S3 shows a STEM-HAADF image of the NiO / LMNO interface, overlaid with regions from which averaged spectra were extracted. The spectra have been aligned to the O $K$ edge at 532 eV to account for energy drift and processed to remove a power law background. As shown on the right side of the figure, there is a clear chemical shift of both the Mn $L_3$ edge ($\Delta = -1.5 \pm 0.1$ eV) and $L_2$ edges ($\Delta = -0.9 \pm 0.1$ eV), which confirms a transition from a $Mn^{4+}$-like to $Mn^{3+}$-like state in the vicinity of the precipitate, in good agreement with our DFT simulations.

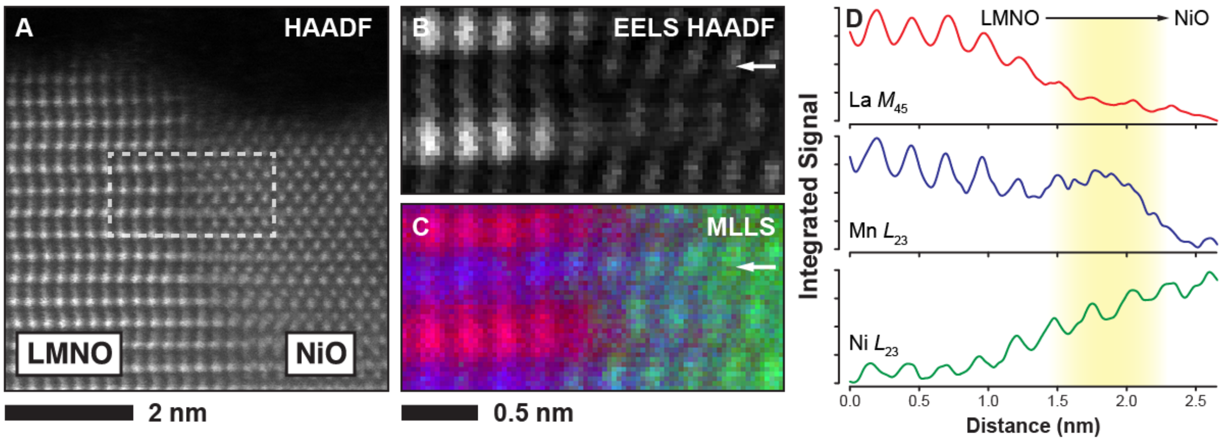


FIG. S2. Local composition mapping in the vicinity of the NiO phase. (A) Overall STEM-HAADF image and (B) region of the EELS map. (C) Corresponding map of the NiO and LMNO phases generated using multiple linear least squares (MLLS) fitting. (D) Integrated signal profiles for the La $M_{4,5}$, Mn $L_{2,3}$, and Ni $L_{2,3}$ edges.

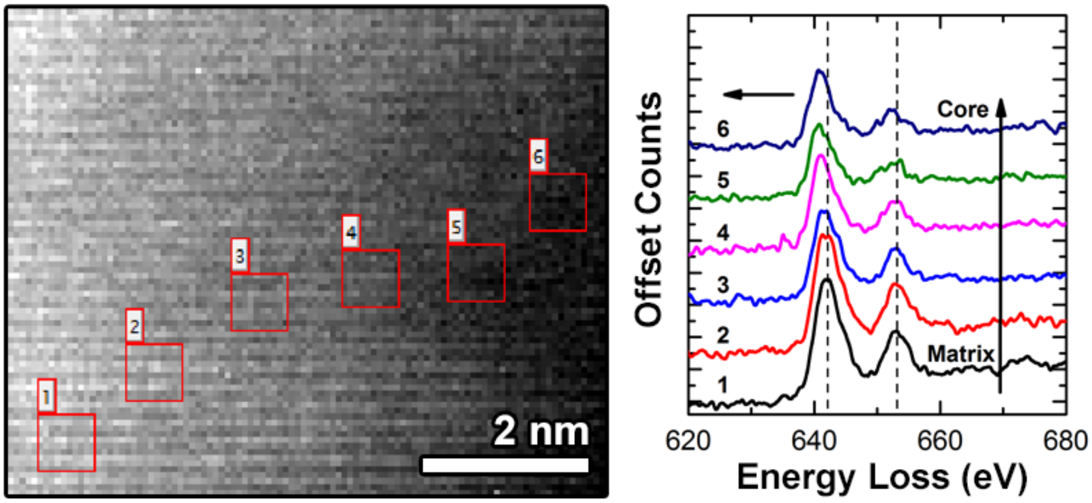


FIG. S3. STEM-EELS mapping of Mn valence in the vicinity of a NiO region. Left: STEM-HAADF region overlaid with regions from which average spectra are taken. Right: Background-subtracted Mn $L_{2,3}$ edge spectra moving from the matrix (region 1) into the NiO precipitate (region 6). The dashed lines have been added as a guide to the eye.

## D. Spatial Distribution of Alloying Elements

As described in the main text, APT datasets containing dozens of NiO precipitates reveal the presence of a defect-free interface layer spanning 1–5 nm adjacent to the STO substrate. Figure S4.A shows another region containing the representative gap between the bottom of the NiO precipitates and the substrate. This behavior is shown more clearly in Figure S4.B, which plots at % line profiles for each of the cation species in the compound. We note the clear absence of any Sr and Ti beyond the marked STO, supporting the presence of an NiO-free region at the film-substrate interface. La/Sr intermixing is only noticeable at the top surface of the STO region. While APT of oxide thin films can provide key compositional information at sub-nm spatial resolution, the absolute measurement of compositional intermixing at the film-substrate interface (∼2 nm around the dashed line) is sensitive to ion trajectory aberrations due to the evaporation field difference between the LMNO and STO. This effect has been described in investigations of $CeO_2$ / $ZrO_2$ multilayers,[12] where it was shown that APT may not give an accurate measure of compositional intermixing at interfaces exhibiting significant field evaporation differences. Thus, the interface profile is likely sharper than measured in APT, as evidenced by the abrupt interfaces in Figure S1.

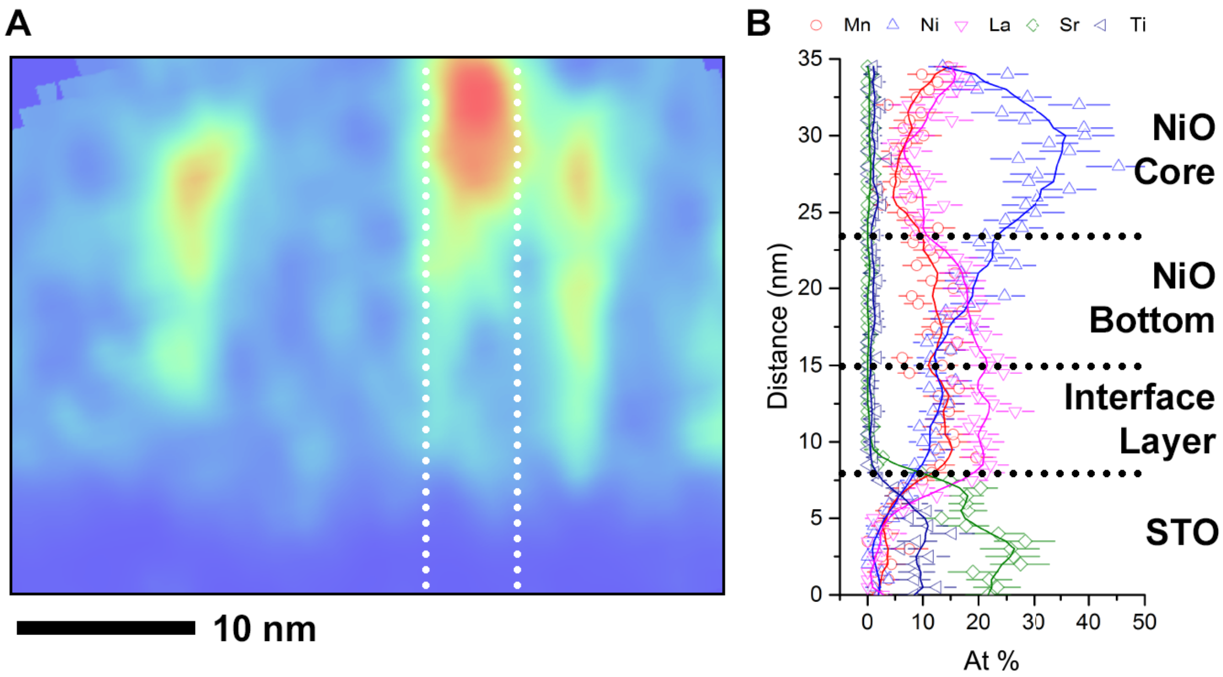


FIG. S4. (A) 2D Ni composition map of another part of the film. Dashed lines indicate the averaging region from which the line profile in (B) was extracted. Raw data points have been overlaid with weighted-average lines. The approximate substrate, interface, and NiO regions are marked with dashed lines.

## E. DFT Calculation Details

Here we provide additional details regarding our simulations of the LMNO structure.

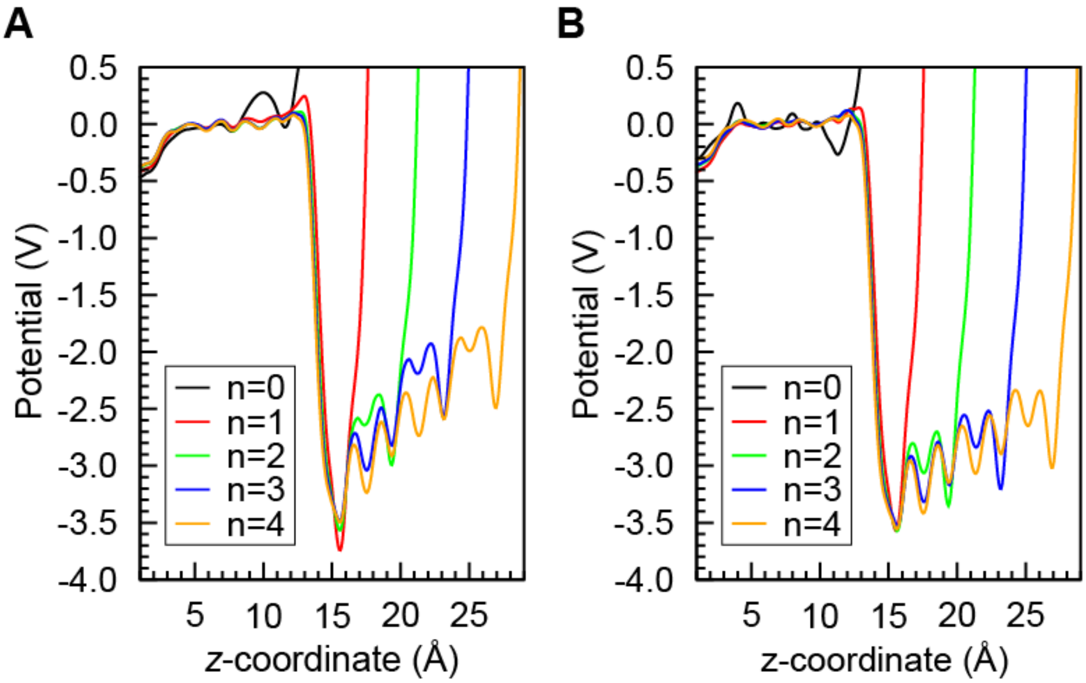


FIG. S5. Electrostatic potential in LMNO ($n$ u.c.) / STO (4 u.c.) as a function of LMNO film thickness $n$. (A) ordered stoichiometric LMNO and (B) LMNO containing a vacancy in the surface $BO_2$ plane.

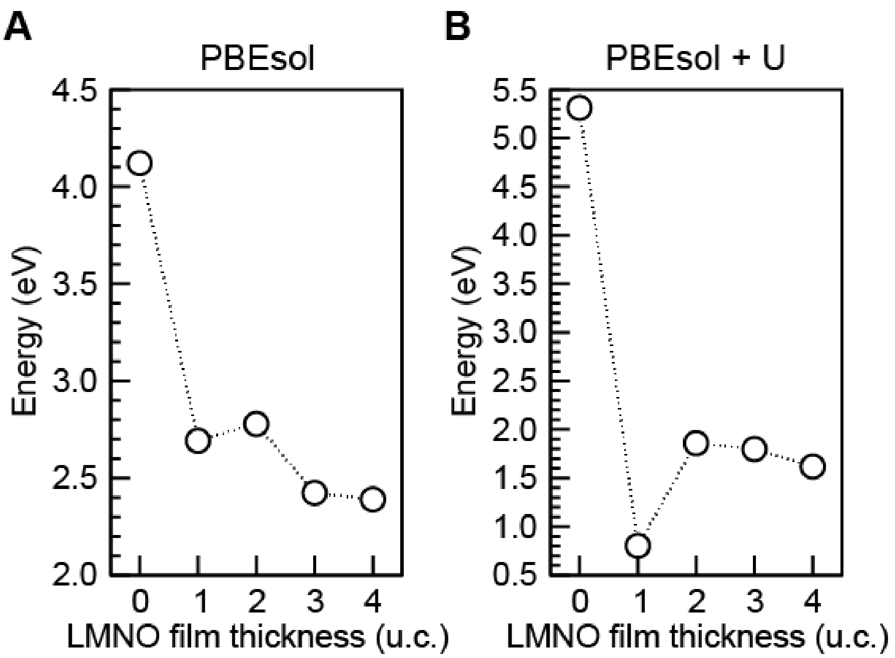


FIG. S6. Formation energies of oxygen vacancies at the surface plane of LMNO / STO as a function of LMNO film thickness, calculated using PBEsol (A) and PBEsol + $U$ (B) functionals with respect to the energy of $O_2$ molecule. PBEsol + $U$ calculations were carried out for the geometrical structures pre-optimized using PBEsol.

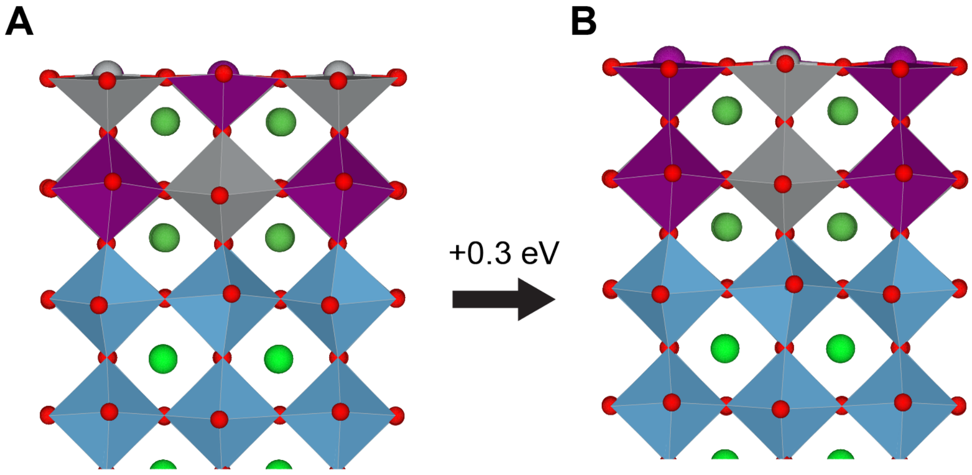


FIG. S7. The ordered stoichiometric LMNO film ($n$ = 2) configuration (A) is 0.3 eV per 2 × 2 lateral cell more stable than the configuration in which the surface $BO_2$ plane is shifted in-plane by a (1/2, 1/2) vector (B), suggesting a high probability of cation defect formation.

TABLE SI. Defect formation energies. $E_{(MnO_2/NiO_2)}$ is the energy cost of segregating the surface LMNO plane into $MnO_2$ and $NiO_2$ phases each having a surface area of 4 u.c. In the Ni-rich case, the energies of forming each sequential vacancy are given.

| $n$ | $E_{(MnO_2/NiO_2)}$ | Formation energies of $V_O$ in the surface $BO_2$ plane | | | | |
|---|---|---|---|---|---|---|
| | per 2×4 u.c. | Ordered | Ni-rich surface plane: $4{\times}NiO_{2-x}$ | | | |
| | | $1{\times}V_O$ | $1^{st}$ $V_O$ | $2^{nd}$ $V_O$ | $3^{rd}$ $V_O$ | $4^{th}$ $V_O$ |
| | | | $x$=0.25 | $x$=0.50 | $x$=0.75 | $x$=1.00 |
| 1 | 1.216 | 2.694 | 1.079 | 2.271 | 2.426 | 2.779 |
| 2 | 0.812 | 2.779 | 1.286 | 2.225 | 1.929 | 3.259 |
| 3 | 0.845 | 2.423 | 1.226 | 1.774 | 1.616 | 3.280 |
| 4 | 0.764 | 2.390 | 1.170 | 1.817 | 1.826 | 2.746 |

## REFERENCES


[1]L. Qiao, T. C. Droubay, T. Varga, M. E. Bowden, V. Shutthanandan, Z. Zhu, T. C. Kaspar, and S. A. Chambers, "Epitaxial growth, structure, and intermixing at the $LaAlO_3$ / $SrTiO_3$ interface as the film stoichiometry is varied," Phys. Rev. B **83**, 085408 (2011).

[2]S. R. Spurgeon, Y. Du, T. Droubay, A. Devaraj, X. Sang, P. Longo, P. Yan, P. G. Kotula, V. Shutthanandan, M. E. Bowden, J. M. LeBeau, C. Wang, P. V. Sushko, and S. A. Chambers, "Competing pathways for nucleation of the double perovskite structure in the epitaxial synthesis of $La_2MnNiO_6$," Chem. Mater. **28**, 3814–3822 (2016).

[3]L. Jones, H. Yang, T. J. Pennycook, M. S. J. Marshall, S. Van Aert, N. D. Browning, M. R. Castell, and P. D. Nellist, "Smart Align—a new tool for robust non-rigid registration of scanning microscope data," Adv. Struct. Chem. Imaging **1**, 8 (2015).

[4]A. Devaraj, D. E. Perea, J. Liu, L. M. Gordon, T. J. Prosa, P. Parikh, D. R. Diercks, S. Meher, R. P. Kolli, Y. S. Meng, and S. Thevuthasan, "Three-dimensional nanoscale characterisation of materials by atom probe tomography," International Materials Reviews **0**, 1–34 (2017).

[5]G. Kresse and D. Joubert, "From ultrasoft pseudopotentials to the projector augmented-wave method," Phys. Rev. B **59**, 1758–1775 (1999).

[6]G. Kresse and J. Furthmüller, "Efficient iterative schemes for ab initio total-energy calculations using a plane-wave basis set," Phys. Rev. B **54**, 11169–11186 (1996).

[7]P. E. Blöchl, "Projector augmented-wave method," Phys. Rev. B **50**, 17953–17979 (1994).

[8]J. P. Perdew, A. Ruzsinszky, G. I. Csonka, O. A. Vydrov, G. E. Scuseria, L. A. Constantin, X. Zhou, and K. Burke, "Restoring the density-gradient expansion for exchange in solids and surfaces," Phys. Rev. Lett. **100**, 136406 (2008).

[9]R. Bader, *Atoms in Molecules A Quantum Theory* (Oxford University Press, Oxford, 1990).

[10]S. L. Dudarev, G. A. Botton, S. Y. Savrasov, C. J. Humphreys, and A. P. Sutton, "Electron-energy-loss spectra and the structural stability of nickel oxide: An LSDA+U study," Phys. Rev. B **57**, 1505–1509 (1998).

[11]A. Floris, S. de Gironcoli, E. K. U. Gross, and M. Cococcioni, "Vibrational properties of MnO and NiO from DFT+U-based density functional perturbation theory," Phys. Rev. B **84**, 161102 (2011).

[12] N. Madaan, J. Bao, M. Nandasiri, Z. Xu, S. Thevuthasan, and A. Devaraj, "Impact of dynamic specimen shape evolution on the atom probe tomography results of doped epitaxial oxide multilayers: Comparison of experiment and simulation," Applied Physics Letters **107**, 091601 (2015).
